# Supplementary material for: RIGID: Recurrent GAN Inversion and Editing of Real Face Videos
Source: arXiv:2308.06097 source file (2023-08-15)
Supplement: Supplementary file 1 [file supp_1.tex]

\begin{figure*}
    \centering
    \subfloat[\footnotesize{Original}]{
    \begin{minipage}{0.19\linewidth}
    \animategraphics[autoplay,loop,width=\textwidth]{24}{figure/edit/IN_THE_WILD_CROP/ORI/jim/}{0100}{0148}\\
    \animategraphics[autoplay,loop,width=\textwidth]{24}{figure/edit/IN_THE_WILD_CROP/ORI/jim/}{0100}{0148}%\\
    \end{minipage}
    }
    \hspace{-2.25mm}
    \subfloat[\footnotesize{IGCI}\label{fig_igci}]{
    \begin{minipage}{0.19\linewidth}
    \animategraphics[autoplay,loop,width=\textwidth]{24}{figure/rec/IN_THE_WILD_CROP/XU/jim/}{0100}{0148}\\
    \animategraphics[autoplay,loop,width=\textwidth]{24}{figure/edit/IN_THE_WILD_CROP/XU/jim_Chubby_rep/}{0100}{0148}%\\
    \end{minipage}
    }
    \hspace{-2.25mm}
    \subfloat[\footnotesize{Latent-T}\label{fig_lt}]{
    \begin{minipage}{0.19\linewidth}
    \animategraphics[autoplay,loop,width=\textwidth]{24}{figure/rec/IN_THE_WILD_CROP/Latent_T/jim/}{0100}{0148}\\
    \animategraphics[autoplay,loop,width=\textwidth]{24}{figure/edit/IN_THE_WILD_CROP/LT/jim_Chubby_rep/}{0100}{0148}%\\
    \end{minipage}
    }
    \hspace{-2.25mm}
    \subfloat[\footnotesize{STIT}\label{fig_stit}]{
    \begin{minipage}{0.19\linewidth}
    \animategraphics[autoplay,loop,width=\textwidth]{24}{figure/rec/IN_THE_WILD_CROP/STIT/jim/}{0100}{0148}\\
    \animategraphics[autoplay,loop,width=\textwidth]{24}{figure/edit/IN_THE_WILD_CROP/STIT/jim_Chubby_rep/}{0100}{0148}%\\
    \end{minipage}
    }
    \hspace{-2.25mm}
    \subfloat[\footnotesize{RIGID}\label{fig_rigid}]{
    \begin{minipage}{0.19\linewidth}
    \animategraphics[autoplay,loop,width=\textwidth]{24}{figure/rec/IN_THE_WILD_CROP/FULL_32/jim/}{0100}{0148}\\
    \animategraphics[autoplay,loop,width=\textwidth]{24}{figure/edit/IN_THE_WILD_CROP/FULL_32/jim_Chubby_rep/}{0100}{0148}%\\
    \end{minipage}
    }
    \rotatebox[origin=c]{270}{ \small{\texttt{+Chubby}} \hspace{-45mm} \small{\texttt{Inversion}}}\\
    % \rotatebox[origin=c]{270}{\hspace{-60mm} \small{\texttt{+Chubby}} \hspace{-50mm} \small{\texttt{Inversion}}}\\

\caption{Comparisons of video inversion and editing with existing methods. Our RIGID achieves temporal coherent inversion and editing performances. IGIC and Latent-Transformer cannot provide consistent results both for inversion and editing. STIT cannot support the ``Chubby'' editing. This figure contains \emph{animated videos}, which are best viewed using Adobe Acrobat.}
\label{fig:qualitative}
% \vspace{-0.75cm}
\end{figure*}
